# Supplementary material for: Disorder-induced Localization in a Strongly Correlated Atomic Hubbard Gas
Source: arXiv:1305.6072 ancillary file (2014-10-03)
Supplement: Supplementary file 1 [file SM_PRL.pdf]

# Supplemental Material for "Disorder-induced Localization in a Strongly Correlated Atomic Hubbard Gas"

S.S. Kondov,[1,*] W.R. McGehee,[1] W. Xu,[1] and B. DeMarco[1]

[1]*Department of Physics, University of Illinois at Urbana-Champaign, Urbana, Illinois 61801, USA*

(Dated: October 3, 2014)

## EXPERIMENTAL DETAILS

We create ultracold gases of $^{40}$K atoms cooled to temperatures below $T_F$ in a crossed-beam 1064 nm optical dipole trap using standard techniques. For the transport data shown in Figs. 2 and 3, we used $(37–49) \times 10^3$ atoms cooled to $(0.16 \pm 0.01)\, T_F$ in the dipole trap. For the data shown in Fig. 4, the number of atoms varied from $(15–38) \times 10^3$. Imaging artifacts such as interference fringes are removed using a background image basis decomposition [1] for all absorption images. The geometric mean $\omega$ of the harmonic trap frequencies is varied across $2\pi \times$ (95–120) Hz and is determined by the dipole trap optical power and a contribution from the profile of the lattice laser beams. The ratio of the overall vertical to horizontal trap frequencies is approximately fixed at 1.6. The characteristic density is given by $\tilde{\rho} = N \left(\frac{m\omega^2 d^2}{12t}\right)^{\frac{3}{2}}$ [2]. For the $N$, $\omega$, and $s$ used in this work, $\tilde{\rho} = 0.6–3.7$ and the central filling varies from 0.3–0.7 particles per site for each spin state in the clean lattice (according to a Hartree-Fock calculation).

The magnitude of the impulse we apply to the gas is chosen so that the maximum quasimomentum of the center-of-mass of the gas is less than $\hbar\pi/2d$, and thus the sign of the dispersion is positive for the COM velocity. Relative displacement between the spin components during the impulse resulting from a slight magnetic-moment mismatch is less than 0.7 $\mu$m, which is small compared with the typical 5 $\mu$m root mean square (RMS) radius of the gas along the impulse direction. The COM velocity without an impulse $v_{res}$ is not zero because of noise in the position of the gas and imaging noise.

The lattice and optical speckle light is superimposed on the atoms over 150 ms, keeping the ratio $\Delta/s$ fixed. The average speckle field intensity is modulated by a Gaussian envelope with a 170 $\mu$m $1/e^2$ radius and is uniform to within a few percent over the gas. The lattice potential depth is calibrated to within 10% systematic uncertainty using lattice modulation, and $\Delta$ is calibrated to within 10% statistical uncertainty by measuring the dipole force from the speckle envelope. There is a systematic uncertainty in $\Delta$ related to measuring the speckle envelope that is less than 40%. Since the speckle field propagates along a non-lattice direction, resulting in a speckle correlation length along all lattice axes comparable to $d$, the Hubbard energies are weakly correlated between adjacent sites and are nearly isotropic in space [3]. The intensity of the speckle is approximately Gaussian correlated, with 310 nm and 1600 nm RMS autocorrelation lengths along the transverse and propagation directions,

respectively.

## THERMODYNAMIC CALCULATIONS

We use a self-consistent, semi-classical Hartree-Fock calculation [4] to estimate temperature, density, and the Fermi energy in the lattice. In this approach, we ignore the fast spatial variation of the speckle and treat the disorder potential as giving rise to an overall chemical potential shift. The central density is overestimated in this approximation because the disorder will exclude atoms from high-speckle-intensity regions of the trap. We calculate the density self-consistently as

$$n(\vec{r}) = \frac{1}{h^3} \int d^3\vec{q}\, \frac{1}{e^{-\beta\mu} e^{\beta[m\omega^2 r^2/2 + \epsilon(\vec{q}) + n(\vec{r})Ud^3]} + 1}, \tag{1}$$

where $\vec{q}$ is the quasimomentum, $\epsilon(\vec{q})$ is the single-particle lattice dispersion, and $\beta = 1/k_B T$. We solve for $\mu$ and $T$ to reproduce the experimental number of atoms and entropy, assuming that tuning on the lattice is isentropic. The entropy is computed from the thermodynamic potential $\Omega$ by $S = -d\Omega/dT$, where

$$\Omega = -\frac{k_B T}{h^3} \int d^3\vec{r} \int d^3\vec{q} \cdot \, Log\left[e^{\beta\mu} e^{-\beta\left[m\omega^2 r^2/2 + \epsilon(\vec{q}) + n(\vec{r})Ud^3\right]} + 1\right]. \tag{2}$$

The number of atoms is determined from

$$N = \frac{1}{h^3} \int d^3\vec{r} \int d^3\vec{q} \cdot \, \frac{1}{e^{-\beta\mu} e^{\beta[m\omega^2 r^2/2 + \epsilon(\vec{q}) + n(\vec{r})Ud^3]} + 1}. \tag{3}$$

The Fermi energy is solved for as the $\mu$ necessary to satisfy Eq. 3 in the $T \to 0$ limit.

The Hartree-Fock approach accounts for interactions at the mean-field level. Correlation effects arising from interactions in the metallic regime can be treated more accurately using a high-temperature series expansion [5]. For the clean lattice, the Hartree-Fock calculation reproduces a temperature about 20% higher than the high-temperature series expansion approach (taking into account the trap using the local density approximation). We cannot compare these methods at our lowest temperatures, which are smaller than $t$, since the high-temperature series expansion fails in this regime.

* Now at: Physics Department, Princeton University, Jadwin Hall, Princeton NJ 08544, USA.

[1] M. Erhard, *Experiments with multi-component Bose-Einstein condensates*, Ph.D. thesis, University of Hamburg (2004).

[2] L. De Leo, C. Kollath, A. Georges, M. Ferrero, and O. Parcollet, Phys. Rev. Lett. **101**, 210403 (2008).

[3] M. White, M. Pasienski, D. McKay, S. Q. Zhou, D. Ceperley, and B. DeMarco, Phys. Rev. Lett. **102**, 055301 (2009).

[4] W. Nolting and W. Brewer, *Fundamentals of Many-body Physics: Principes and Methods* (Springer, 2009).

[5] V. W. Scarola, L. Pollet, J. Oitmaa, and M. Troyer, Phys. Rev. Lett. **102**, 135302 (2009).
